# Supplementary material for: DISK: Differentiable Sparse Kernel Complex for Efficient Spatially-Variant Convolution
Source: arXiv:2512.04556 source file (2026-05-19)
Supplement: Supplementary file 1 [file supp.tex]

\appendix
\section{Sampling Algorithm of Kernel Shape}
\begin{algorithm}[H]
\caption{Non-Convex Kernel Initialization via Rejection Sampling}
\label{alg:rejection-sampling}
\begin{algorithmic}[1]
\STATE \textbf{Input:} Target kernel $K$, Number of samples $N_s$
\STATE \textbf{Output:} Initial offsets for the first sparse kernel $O_0$
\STATE $M \gets \text{Coordinates of non-zero pixels in } K$
\STATE $S \gets |M|$
\STATE $r \gets \sqrt{S / (N_s \cdot \pi)}$ \COMMENT{Initial rejection radius}
\STATE $O_0 \gets \emptyset$ \COMMENT{Initialize empty set for offsets}

% \IF{$\text{each candidate coordinate } p \in M$}
\FOR{each candidate coordinate $p \in M$} 
    \IF{$|O_0| \ge N_s$} 
        \STATE \textbf{break}
    \ENDIF
    \IF{$\forall o \in O_0, \| p - o \| \ge r$}
        \STATE $O_0 \gets O_0 \cup \{p\}$ \COMMENT{Accept sample if it's not too close to others}
    \ENDIF
\ENDFOR

\IF{$|O_0| < N_s$}
    \STATE $N_{\text{rem}} \gets N_s - |O_0|$ \COMMENT{Handle case where not enough samples were found}
    \STATE $M_{\text{fill}} \gets \text{First } N_{\text{rem}} \text{ coordinates from a deterministic repetition of } M$
    \STATE $O_0 \gets O_0 \cup M_{\text{fill}}$
\ENDIF
\STATE $O_0 \gets O_0 - \text{center}(K)$ \COMMENT{Center the offsets}
\STATE \textbf{return} $O_0$
% \Return $O_0$
\end{algorithmic}
\end{algorithm}
\section{Additional Result}
\subsection{Ablation on multiple configs of samples and layers}
\chg{We present ablation of samples and layers on another kernel, \emph{Dove}, in~\refFig{fig:layer-abl-dove}.}
\begin{figure}[htb]
    \centering
    \begin{minipage}{0.38\columnwidth} % 调整宽度，确保两张图能并排显示
        \centering
        \includegraphics[width=\linewidth]{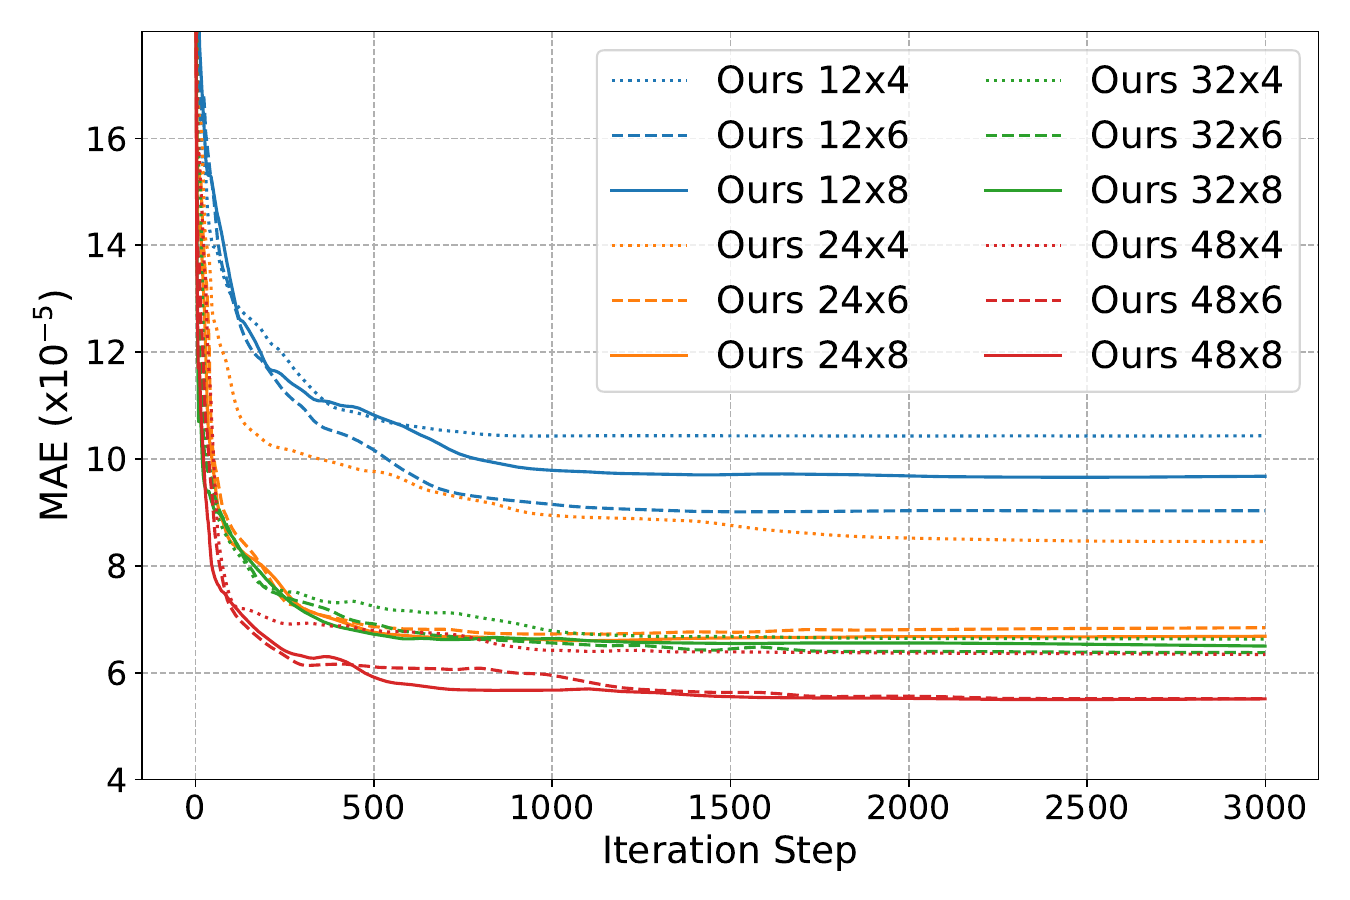}
    \end{minipage}
    \hfill 
    \begin{minipage}{0.3\columnwidth} % 调整宽度，确保两张图能并排显示
        \centering
        \vspace{-6pt}
        \includegraphics[width=\linewidth]{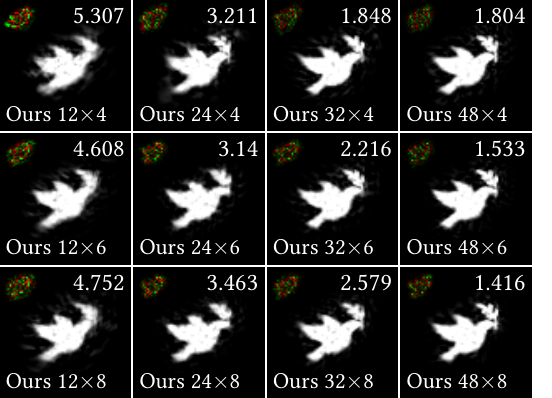}
    \end{minipage}
    \begin{minipage}{0.3\columnwidth} % 调整宽度，确保两张图能并排显示
        \centering
        \vspace{-6pt}
        \includegraphics[width=\linewidth]{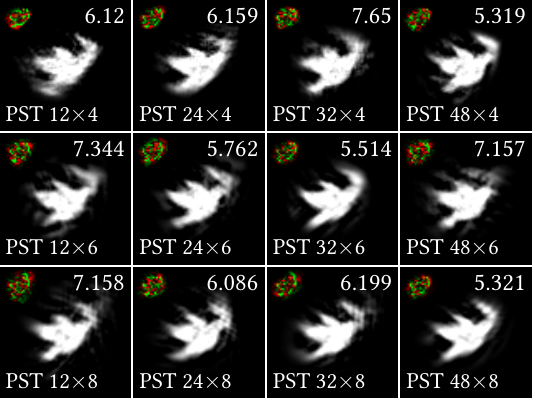}
    \end{minipage}
    \caption{Ablation results for various configurations of samples and layers on \emph{Dove} kernel.}
    \label{fig:layer-abl-dove}
\end{figure}
\subsection{Ablation on Gaussian Kernel of Fewer Samples}
For symmetric targets like Gaussians, we enforce a Kawase-like (KWS) symmetry constraint on the sampling offsets. Table~\ref{tab:ablation-gaussian} shows this constraint consistently improves results, proving particularly effective when using only a few samples per layer. We also found that an L1 loss on the impulse response is substantially more effective than an L2 loss for this task. Our final model for Gaussian kernels with fewer samples (e.g., 6-layer and 4 samples per layer) can combine an L1 loss with symmetry constraint and IR strategies.
\begin{table}[htb]
\centering
\small % 调小一级字号
\setlength{\tabcolsep}{1.0pt} % 缩小列间距
\caption{Ablation results of filtering of Gaussian kernels on impulse response.}
\label{tab:ablation-gaussian}
% 1 (Variant) + 3 (gs5) + 3 (gs7) + 3 (gs9) + 3 (gs11) = 13 columns
\begin{tabular}{lcccccccccccc} % 'l' for the first column, 'c' for the rest
\toprule
\multirow{2}{*}{\diagbox{Variant}{Filter}} & \multicolumn{3}{c}{$\sigma=5$} & \multicolumn{3}{c}{$\sigma=7$} & \multicolumn{3}{c}{$\sigma=9$} & \multicolumn{3}{c}{$\sigma=11$} \\
\cmidrule(lr){2-4} \cmidrule(lr){5-7} \cmidrule(lr){8-10} \cmidrule(lr){11-13}
& PSNR$\uparrow$ & LPIPS$\downarrow$ & FLIP$\downarrow$ & PSNR$\uparrow$ & LPIPS$\downarrow$ & FLIP$\downarrow$ & PSNR$\uparrow$ & LPIPS$\downarrow$ & FLIP$\downarrow$ & PSNR$\uparrow$ & LPIPS$\downarrow$ & FLIP$\downarrow$ \\
\midrule
L1+KWS+IR  & 97.79 & \textbf{.0099} & \textbf{.2604} & \textbf{99.98} & \textbf{.0052} & \textbf{.4943} & \textbf{99.85} & \textbf{.0028} & \textbf{.1906} & \textbf{96.77} & \textbf{.0063} & \textbf{.3926} \\
L1+KWS+R    & 96.11 & .0150 & .5567 & 93.46 & .0181 & .6603 & 90.57 & .0256 & .4152 & 79.72 & .2737 & 2.670 \\
L1+IR           & \textbf{98.31} & .0117 & .3871 & 93.69 & .0394 & .7209 & 91.83 & .1142 & .9803 & 91.99 & .0942 & .7191 \\
L1+R        & 97.64 & .0191 & .4443 & 93.05 & .0705 & .7021 & 90.77 & .1606 & .9916 & 88.16 & .3198 & 1.226 \\
L2+KWS+IR  & 65.04 & 19.57 & 6.635 & 67.77 & 1.393 & 7.119 & 69.96 & .3123 & 7.156 & 71.80 & .1318 & 6.576 \\
L2+Inc       & 90.18 & .0849 & .8460 & 90.02 & .1433 & 1.066 & 83.84 & .2396 & 2.291 & 77.17 & .4472 & 4.389 \\
\bottomrule
\end{tabular}
\end{table}

\subsection{Initialization ablation on various kernels}
As shown in Table~\ref{tab:ablation-arbitrary}, a basic random initialization performs poorly. Using either our sparse sampling (SS) for the first layer or our increasing-step radial initialization (IR) for all layers provides a significant boost, but combining them as SS+IR is critical for achieving the best performance. This confirms our hypothesis that a hybrid strategy is optimal, with SS capturing kernel shape and IR ensuring stable receptive field growth. Furthermore, weight normalization is crucial; both sum-to-one (SUM) and softmax (SOFM) are effective, with SUM holding a slight, consistent advantage.  
\begin{table}[htb]
\centering
\small % 调小一级字号
\setlength{\tabcolsep}{2.5pt} % 缩小列间距
\caption{\textbf{Ablation on arbitrary kernels.} Our full model (SUM+SS+IR) achieves the best performance. SUM/SOFM: sum-to-one/softmax weight normalization. SS: sparse sampling initialization. IR/R: increasing/fixed-step radial initialization. Basic: random initialization. \chg{For LPIPS and FLIP scores, both lower is better.}}
\label{tab:ablation-arbitrary}
\begin{tabular}{lcccccccccccccccc} % 'l' for the first column, 'c' for the rest
\toprule
\multirow{2}{*}{\diagbox{Variant}{Filter}} & \multicolumn{2}{c}{\small Ampersand} & \multicolumn{2}{c}{Disk} & \multicolumn{2}{c}{Heart} & \multicolumn{2}{c}{Star4} & \multicolumn{2}{c}{Ring} & \multicolumn{2}{c}{4-Sided} & \multicolumn{2}{c}{6-Sided} & \multicolumn{2}{c}{Star} \\
\cmidrule(lr){2-3} \cmidrule(lr){4-5} \cmidrule(lr){6-7} \cmidrule(lr){8-9} \cmidrule(lr){10-11} \cmidrule(lr){12-13} \cmidrule(lr){14-15} \cmidrule(lr){16-17}
& \tiny LPIPS & \tiny FLIP & \tiny LPIPS & \tiny FLIP & \tiny LPIPS & \tiny FLIP & \tiny LPIPS & \tiny FLIP & \tiny LPIPS & \tiny FLIP & \tiny LPIPS & \tiny FLIP & \tiny LPIPS &  \tiny FLIP & \tiny LPIPS & \tiny FLIP \\
\midrule
SUM+SS+IR & \textbf{1.44} & 2.63 & \textbf{.240} & 3.53 & \textbf{.230} & 1.54 & .326 & \textbf{3.00} & \textbf{.426} & \textbf{2.46} & \textbf{.276} & \textbf{.375} & \textbf{.218} & \textbf{1.77} & .790 & \textbf{5.28} \\
SOFM+SS+IR & 2.39 & \textbf{2.61} & .242 & 3.54 & .248 & 1.58 & \textbf{.311} & 3.07 & .432 & 2.72 & .299 & .420 & .246 & 2.04 & .798 & 5.38 \\
SUM+SS+R & 1.94 & 3.12 & .251 & \textbf{3.48} & .236 & 1.50 & .386 & 3.48 & .441 & 2.60 & .285 & .492 & .336 & 2.10 & \textbf{.748} & 5.60 \\
SOFM+SS+R & 1.90 & 2.97 & .269 & 3.81 & .241 & \textbf{1.41} & .466 & 3.38 & .434 & 2.48 & .332 & .481 & .374 & 2.67 & .937 & 5.93 \\
SUM+R & 9.74 & 11.7 & .774 & 14.6 & 1.13 & 8.78 & 1.52 & 8.88 & 2.57 & 25.0 & 1.65 & 5.06 & .960 & 10.4 & 6.44 & 11.1 \\
SOFM+R & 9.70 & 11.7 & .773 & 14.6 & 1.13 & 8.78 & 1.52 & 8.88 & 2.57 & 25.0 & 1.65 & 5.06 & .961 & 10.4 & 6.44 & 11.0 \\
SS & 10.4 & 10.3 & .524 & 22.6 & .906 & 11.2 & 2.16 & 15.1 & 2.28 & 10.3 & 1.20 & 12.8 & .744 & 12.6 & 4.62 & 7.61 \\
Basic & 21.1 & 25.3 & 12.0 & 32.8 & 13.9 & 26.7 & 23.2 & 17.3 & 233 & 38.4 & 11.3 & 23.1 & 9.83 & 29.1 & 13.8 & 18.8 \\
\bottomrule
\end{tabular}
\end{table}

\subsection{Single Kernel Comparison}
\chg{We present additional results on single-kernel synthesis in~\refFig{fig:single-kernel-comparison-supp}. We include a diverse set of point-spread functions, ranging from basic depth-of-field bokeh shapes (\emph{Side4}, \emph{Side6}, \emph{Ring}) to more complex geometric silhouettes (\emph{Heart}, \emph{Star4}), an artificial font-based shape (\emph{Ampersand}), and finally dove- and flower-shaped apertures and an optical PSF with spherical aberration. This progression illustrates that our sparse kernels can handle both simple analytic shapes and highly non-Gaussian, visually intricate kernels. We also compare three configurations of our method (32$\times$4, 24$\times$4, and 12$\times$4); while 32$\times$4 generally provides the best reconstruction quality, the 12$\times$4 variant still recovers the main structures despite using very few samples, indicating that our representation retains reasonable expressive power even under an extremely small sample budget.}

\begin{figure}[htb]
    \centering
    \includegraphics[width=\columnwidth]{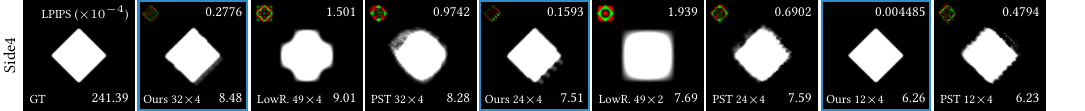}
    \includegraphics[width=\columnwidth]{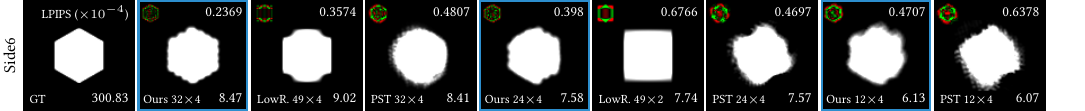}
    \includegraphics[width=\columnwidth]{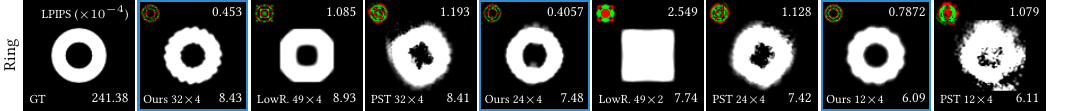}
    \includegraphics[width=\columnwidth]{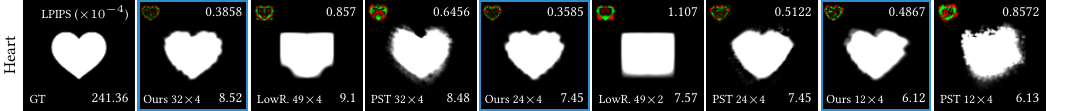}
    \includegraphics[width=\columnwidth]{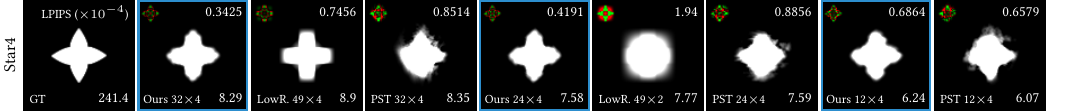}
    \includegraphics[width=\columnwidth]{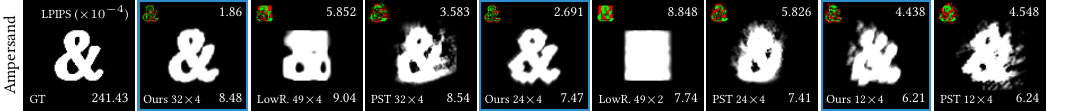}
    \includegraphics[width=\columnwidth]{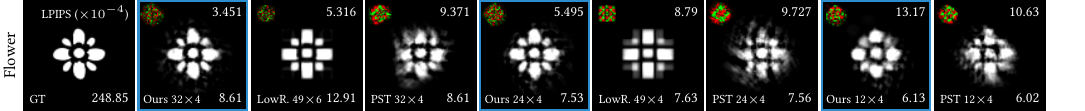}
    \includegraphics[width=\columnwidth]{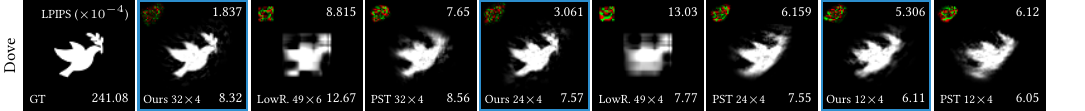}
    \includegraphics[width=\columnwidth]{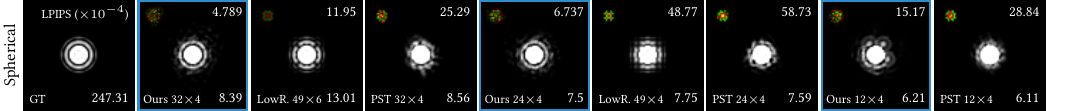}
    \caption{Additional comparison of the single, arbitrary kernels.}
    \label{fig:single-kernel-comparison-supp}
\end{figure}
\subsection{Comparison on Spatial Varying Filtering}
We quantitatively evaluate our filter-space interpolation in~\refFig{fig:sv-lines}, plotting LPIPS error against a continuous kernel size parameter. For all tested kernel shapes, our method achieves lower error than both baselines. The LowRank method is not well-suited for this continuous approximation task, as it exhibits high error across all sizes. The PST baseline is more competitive but remains consistently less accurate than our approach, particularly as the kernel size increases.
\begin{figure}[h]
    \centering
    \includegraphics[width=\columnwidth]{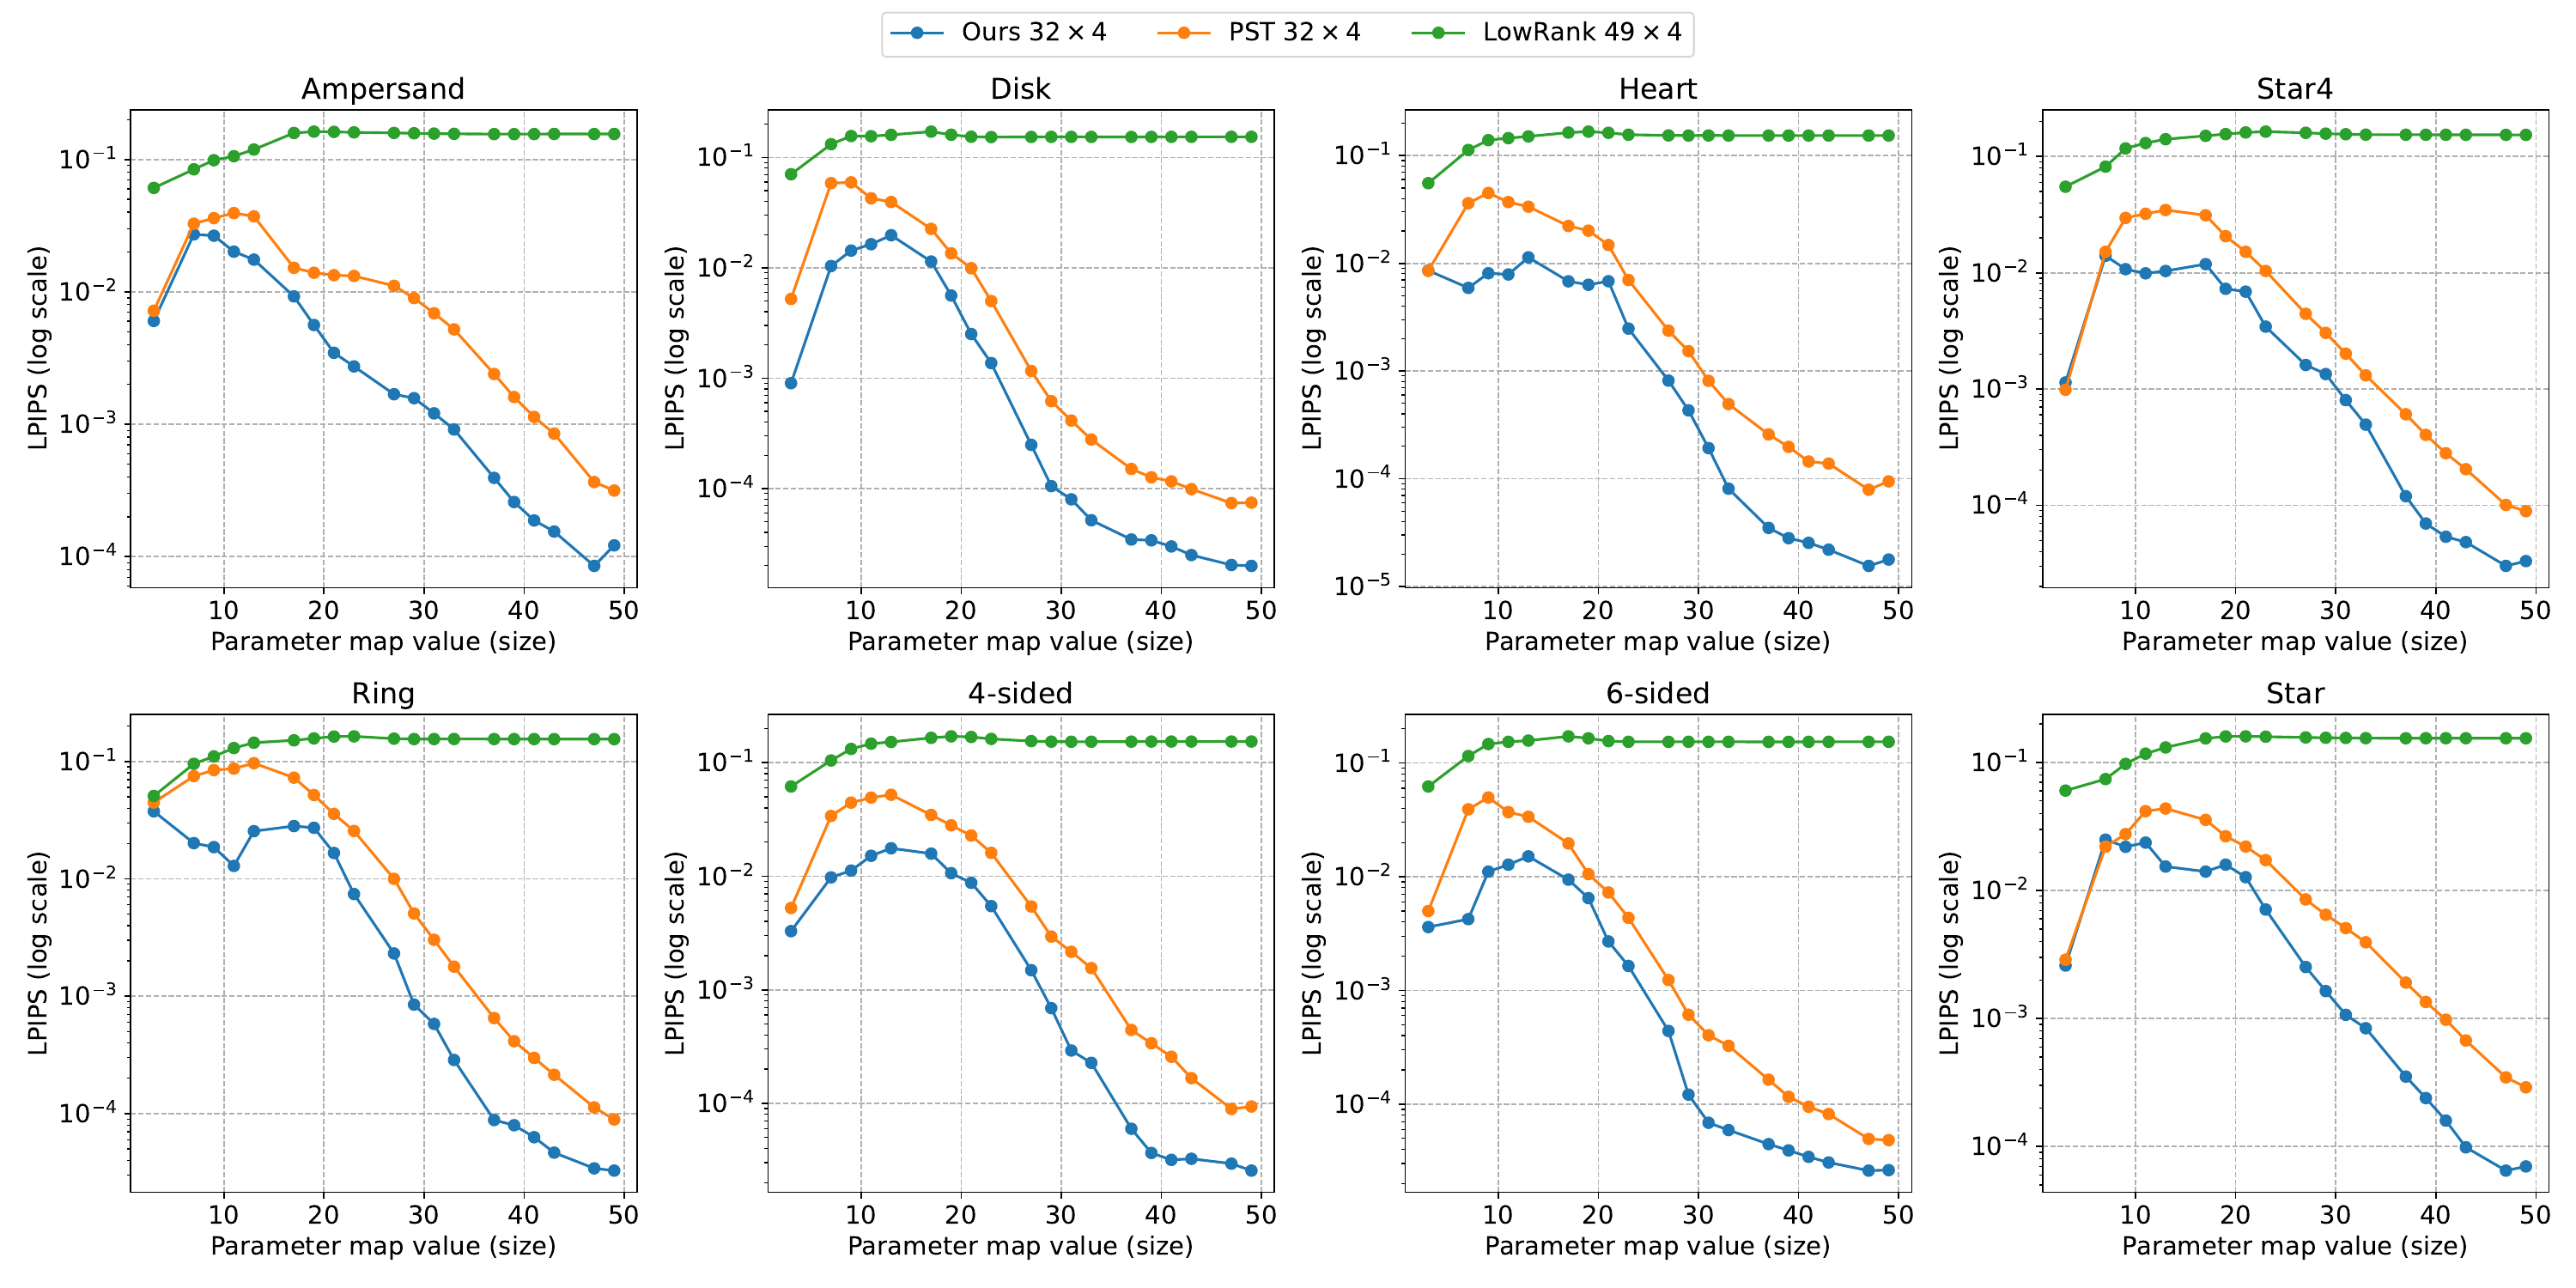}
    \caption{\textbf{Quantitative evaluation of spatially-varying kernel approximation.} We plot LPIPS error (Y-axis, log scale, lower is better) against a continuous kernel size parameter (X-axis) for eight different kernel shapes.}
    \label{fig:sv-lines}
\end{figure}

\subsection{Memory Consumption Analysis}
\chg{We report the memory read and write bandwidth, along with their relative overhead compared to directly displaying the input image, in Table~\ref{tab:memory}. All measurements are collected on a Snapdragon 8 Gen 3 mobile platform at a resolution of $1264\times 2665$.}
\begin{table*}[h]
\centering
\small 
\setlength{\tabcolsep}{2.2pt} 
\caption{\textbf{Memory bandwidth and runtime comparison.} \chg{RB and WB denote read and write bandwidth (MB/frame), while RR and WR represent the \emph{relative increase} in bandwidth with respect to the \emph{Identical} (point sampling) baseline, rather than the raw ratio. Time indicates per-frame runtime (ms). The superscript $^{\star}$ marks 1D spatially varying (SV) kernels. $S\times P$ implies $S$ samples across $P$ passes.}}
\label{tab:memory}
\begin{tabular}{l *{12}{c}}
\toprule
& $\text{Identical}$ & $\text{GT}^{\star}$ & $24\times4^{\star}$ & $32\times4^{\star}$ & $49\times4^{\star}$ & $\text{GT}$ & $12\times4$ & $24\times4$ & $32\times4$ & $49\times2$ & $49\times4$ & $49\times6$ \\
\midrule
$\text{RB}$   & 31.68 & 67.75 & 53.47 & 52.92 & 49.99 & 66.83 & 44.31 & 47.97 & 43.95 & 37.90 & 42.11 & 48.52 \\
$\text{WB}$   & 25.63 & 90.27 & 41.56 & 41.56 & 39.92 & 89.17 & 29.11 & 32.52 & 28.20 & 30.62 & 33.10 & 35.16 \\
$\text{RR}($\%$)$   & 0     & 113.8 & 68.78 & 67.05 & 57.80 & 110.9 & 72.88 & 87.16 & 71.48 & 47.87 & 64.30 & 89.31 \\ 
$\text{WR}($\%$)$   & 0     & 252.2 & 62.15 & 62.15 & 55.75 & 247.9 & 13.58 & 26.88 & 10.03 & 19.47 & 29.15 & 37.18 \\
$\text{Time}$ & 1.04  & 192.4 & 12.66 & 16.78 & 23.29 & 246.8 & 6.13  & 7.50  & 8.36  & 7.72  & 9.11  & 12.56 \\
\bottomrule
\end{tabular}
\end{table*}

\subsection{Comparison to Dilated Convolutions and U-Nets}
~\refFig{fig:single-kernel-cnn-comparison-supp} compares our sparse kernel representation to dilated convolutions and U-Nets for single-kernel synthesis. For the CNN baselines, we reduce the learning rate to one-tenth of ours and increase the number of iterations from 3k to 10k to improve stability. 
% Under these settings, the dilated-convolution models struggle to capture both the wide support and fine details of the highly non-Gaussian PSFs (e.g., \emph{Spherical} and \emph{Coma}), and the U-Nets either oversmooth the structure or introduce visible artifacts. 
Overall, our sparse kernels achieve comparable or lower LPIPS errors with substantially fewer parameters, suggesting that flexible sampling locations are important for representing such complex PSFs.

\begin{figure}[h]
    \centering
    \includegraphics[width=0.8\columnwidth]{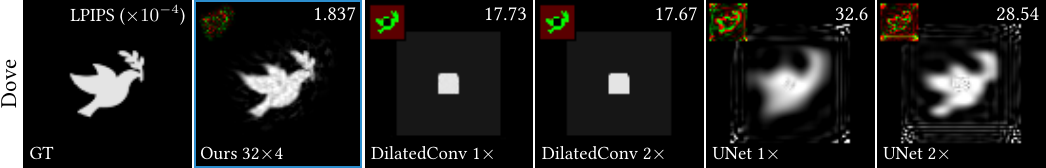}
    \includegraphics[width=0.8\columnwidth]{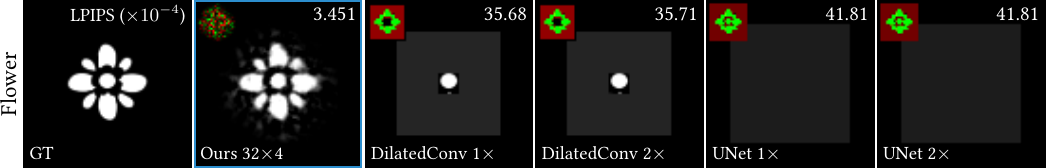}
    \includegraphics[width=0.8\columnwidth]{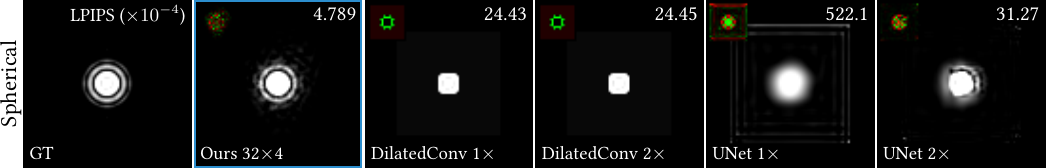}
    \includegraphics[width=0.8\columnwidth]{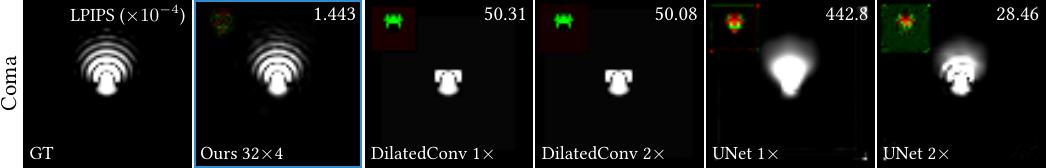}
    \caption{\textbf{Comparison of sparse kernels to CNN baselines on single-kernel synthesis.} \chg{For four representative non-Gaussian PSFs (Dove, Flower, Spherical, and Coma), we show the ground-truth kernel and the reconstructions produced by our sparse kernel (Ours $32\times4$), two dilated-convolution networks, and two U-Nets. Numbers in the top-left of each panel denote LPIPS error ($\times 10^{-4}$, lower is better). The number of trainable parameters is 384 for Ours $32\times4$, 75{,}073 for DilatedConv 1$\times$, 297{,}601 for DilatedConv 2$\times$, 7{,}705 for U-Net 1$\times$, and 17{,}254 for U-Net 2$\times$.}}
    \label{fig:single-kernel-cnn-comparison-supp}
\end{figure}
