# Supplementary material for: DISK: Differentiable Sparse Kernel Complex for Efficient Spatially-Variant Convolution
Source: arXiv:2512.04556 source file (2026-05-19)
Supplement: Supplementary file 2 [file single-kernel-cnn-comparison-supp.tex]

\begin{figure}[h]
    \centering
    \includegraphics[width=0.8\columnwidth]{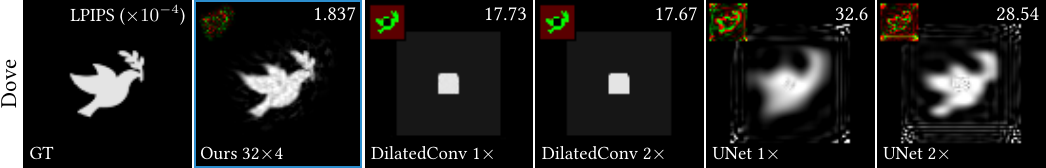}
    \includegraphics[width=0.8\columnwidth]{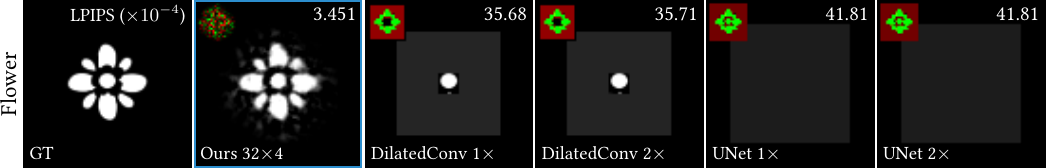}
    \includegraphics[width=0.8\columnwidth]{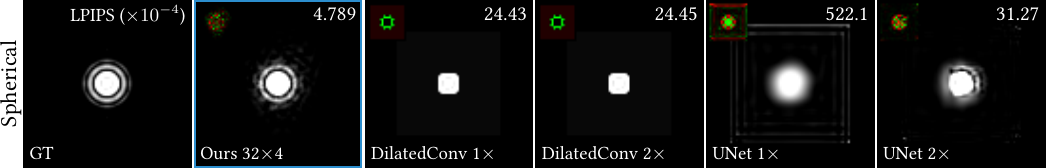}
    \includegraphics[width=0.8\columnwidth]{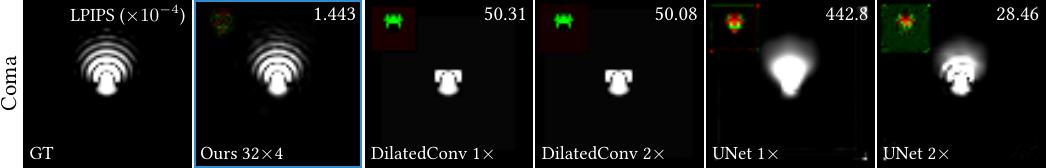}
    \caption{\textbf{Comparison of sparse kernels to CNN baselines on single-kernel synthesis.} \chg{For four representative non-Gaussian PSFs (Dove, Flower, Spherical, and Coma), we show the ground-truth kernel and the reconstructions produced by our sparse kernel (Ours $32\times4$), two dilated-convolution networks, and two U-Nets. Numbers in the top-left of each panel denote LPIPS error ($\times 10^{-4}$, lower is better). The number of trainable parameters is 384 for Ours $32\times4$, 75{,}073 for DilatedConv 1$\times$, 297{,}601 for DilatedConv 2$\times$, 7{,}705 for U-Net 1$\times$, and 17{,}254 for U-Net 2$\times$.}}
    \label{fig:single-kernel-cnn-comparison-supp}
\end{figure}
