# Supplementary material for: DISK: Differentiable Sparse Kernel Complex for Efficient Spatially-Variant Convolution
Source: arXiv:2512.04556 source file (2026-05-19)
Supplement: Supplementary file 3 [file single-kernel-comparison-supp.tex]

\begin{figure}[htb]
    \centering
    \includegraphics[width=\columnwidth]{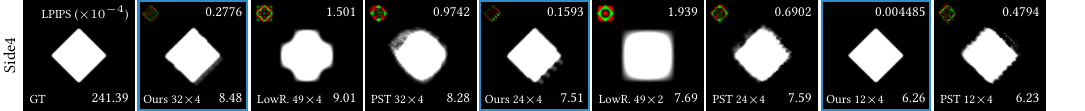}
    \includegraphics[width=\columnwidth]{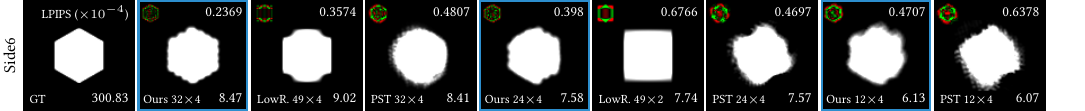}
    \includegraphics[width=\columnwidth]{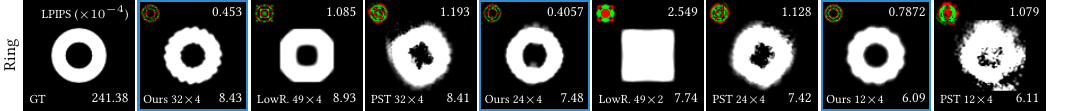}
    \includegraphics[width=\columnwidth]{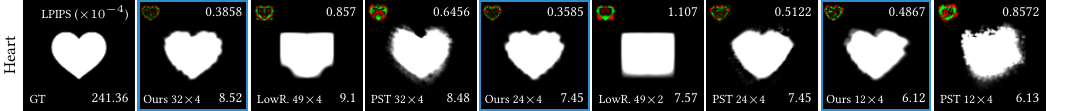}
    \includegraphics[width=\columnwidth]{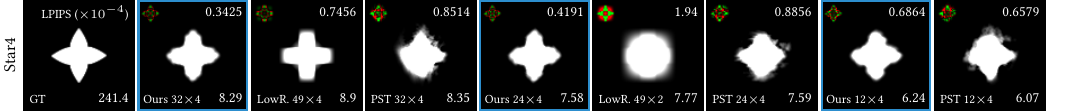}
    \includegraphics[width=\columnwidth]{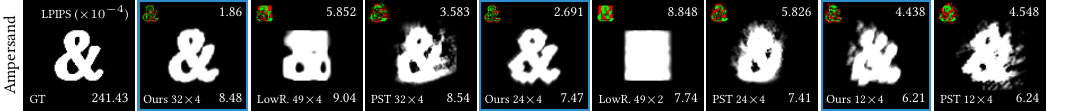}
    \includegraphics[width=\columnwidth]{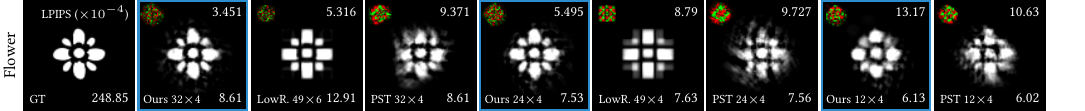}
    \includegraphics[width=\columnwidth]{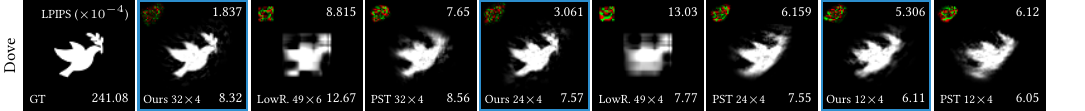}
    \includegraphics[width=\columnwidth]{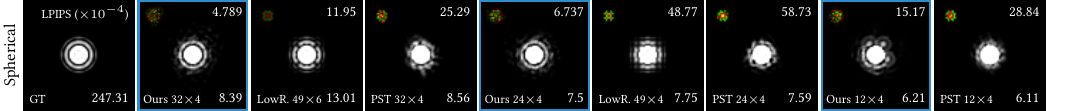}
    \caption{Additional comparison of the single, arbitrary kernels.}
    \label{fig:single-kernel-comparison-supp}
\end{figure}
